# Supplementary material for: Ab initio investigation of H-bond disordering in $\delta$-AlOOH
Source: arXiv:2112.11369 ancillary file (2022-04-25)
Supplement: Supplementary file 1 [file SI.pdf]

# *Ab initio* investigation of H-bond disordering in δ-AlOOH

**Supplementary Information**

Chenxing Luo[1], Koichiro Umemoto[2,3], Renata M. Wentzcovitch[1,4,5,*]

[1] *Department of Applied Physics and Applied Mathematics, Columbia University, New York, NY 10027, USA*
[2] *Earth-Life Science Institute, Tokyo Institute of Technology, Tokyo, Japan*
[3] *Theoretical Quantum Physics Laboratory, Cluster for Pioneering Research, RIKEN, Wako-shi, Saitama 351-0198, Japan*
[4] *Department of Earth and Environmental Sciences, Columbia University, New York, NY 10027, USA*
[5] *Lamont–Doherty Earth Observatory, Columbia University, Palisades, NY 10964, USA*

[*] Corresponding author at Lamont-Doherty Earth Observatory, Columbia University in the City of New York, 61 Route 9W, Palisades, NY 10964, USA. E-mail address: rmw2150@columbia.edu (R.M. Wentzcovitch).

The supporting information consists of Figures S1–S5 and Table S1.

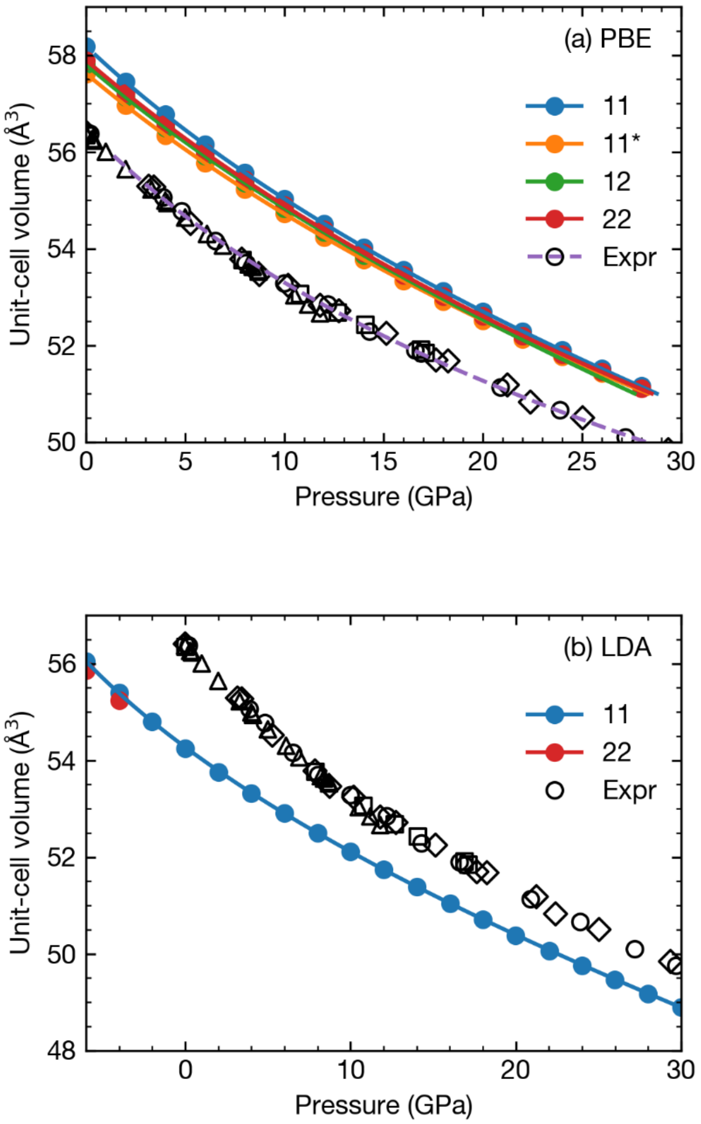


FIG. S1. Static a) PBE and b) LDA compression curves of HOC supercells compared to the 300 K data. Colored curves indicate static results fitted to the third-order B-M finite strain equation of states. Experimental data by Sano-Furukawa et al. [1] are the circles, by Kuribayashi et al. [2] are triangles, by Suzuki [3] are squares, and by Simonova et al. [4] are diamonds. Because (i) the experimental data show good consistency, and (ii) change in compressibility occurs at 8 GPa, fitting the data with a single equation of state was inappropriate, but (iii) no abrupt change in $V$ was observed at this pressure, therefore, a single spline curve (purple dashed curve) was used to fit experimental data. Static PBE calculations show an overall overestimation of ~5 GPa in pressure or ~1.8 Å$^3$ in volume.

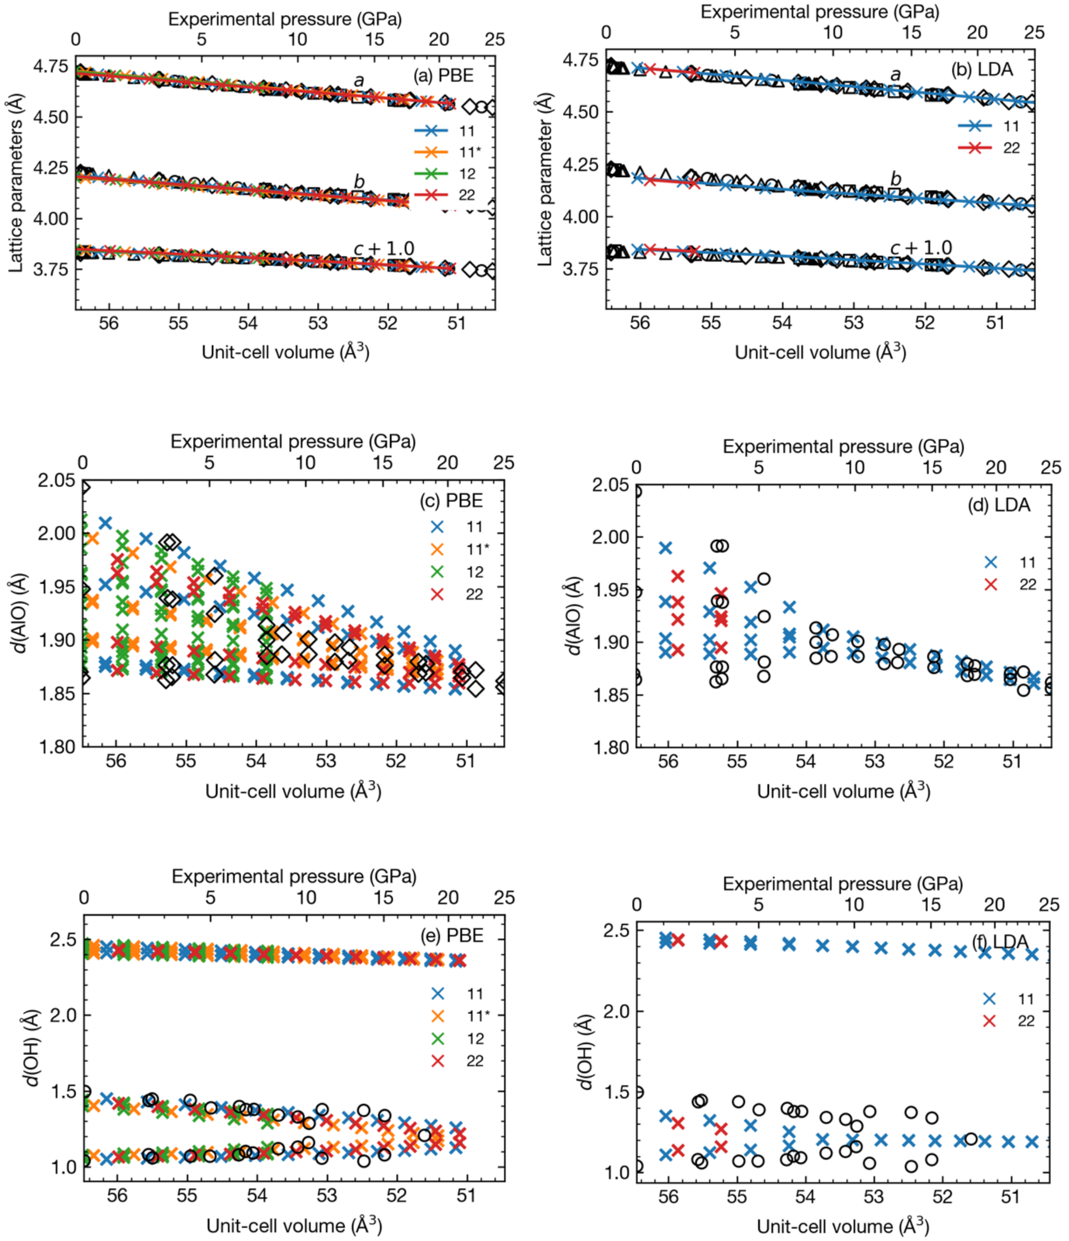


FIG. S2. Comparison between 300 K measured (open black symbols) and (a, c, e) PBE and (b, d, f) LDA results for (a, b) *a*, *b*, *c* lattice parameters, (c, d) *d*(AlO) interatomic distances, and (e, f) *d*(OH) distances vs. volume. Experimental data in (a, b) is from Sano-Furukawa et al. [1] (circles), Kuribayashi et al. [2] (triangles), Suzuki [3] (squares), and Simonova et al. [4] (diamonds); experimental data in (c, d) is from Simonova et al. [4]; experimental

data in (e, f) is from [5]. This type of comparison reveals eventual shortcomings of the exchange-correlation approximations used in the calculations.

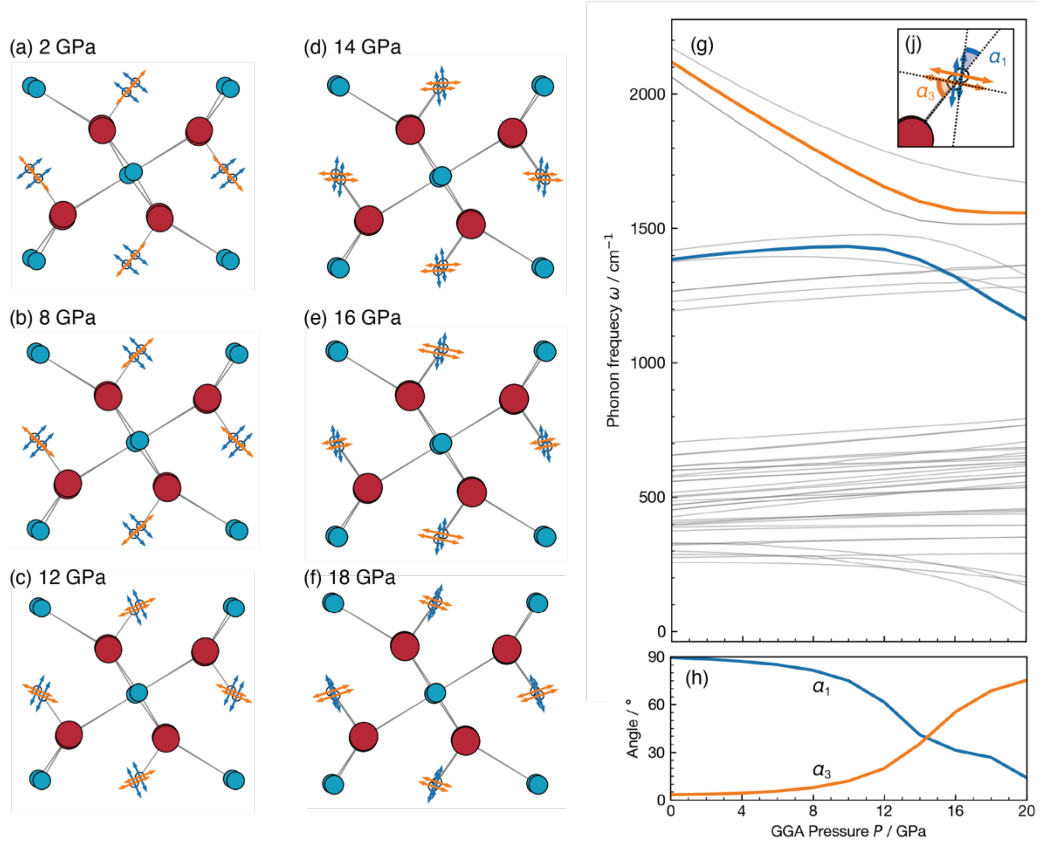


FIG. S3. (a–f) Pressure dependence of atomic displacements associated with two OH modes in the HOC-11* structure. Blue, red, and white spheres denote Al, O, and H ions, respectively. Blue and yellow arrows show atomic displacements associated with modes with highlighted frequencies in (g) with corresponding colors. At low pressures, these modes can be clearly defined as "stretching" (orange) and "bending" (blue) O-H modes where the displacement vector of H ions is parallel ($\alpha_3 = 0°$) and perpendicular ($\alpha_3 = 90°$) to the OH ionic bond directions, respectively. As can be seen in (h), with increasing pressure, these assignments become invalid, but at 18 GPa$^{PBE}$ they recover their "stretching" and "bending" nature but switch the frequency order.

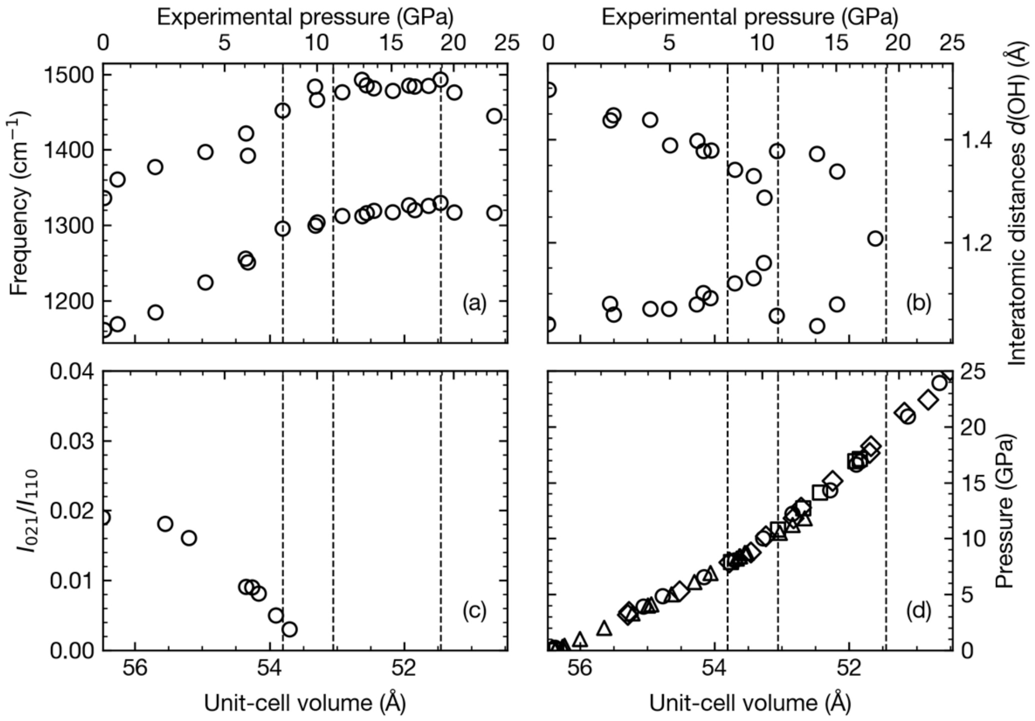


FIG. S4. Pressure/volume dependence at 300 K of measured (a) OH-bending mode frequency [6]; (b) *d*(OH) interatomic distance [5]; (c) relative neutron diffraction peak intensity $I_{021}/I_{110}$ [5]; (d) pressure vs. volume relation from from Sano-Furukawa et al. [1] (circles), by Kuribayashi et al. [2] (triangles), Suzuki [3] (squares), and Simonova et al. [4] (diamonds). Dashed vertical lines denote our proposed boundary between stages of the transition sequence.

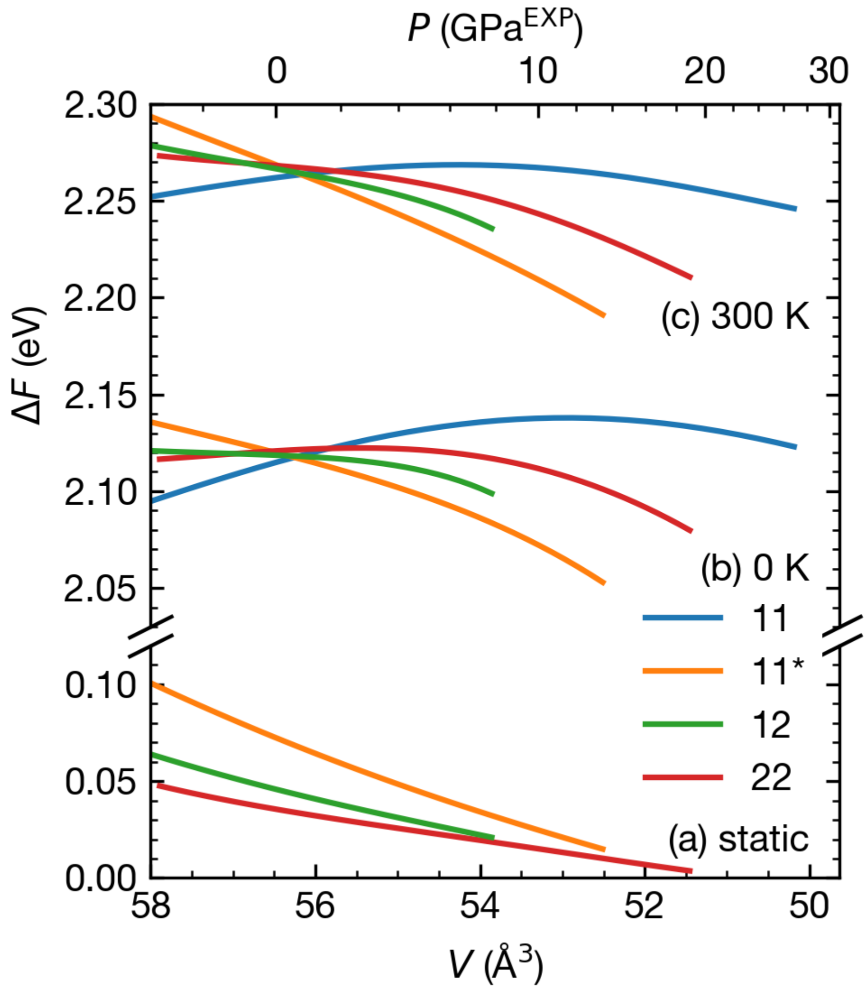


FIG. S5. Energy difference w.r.t. static energy of the HOC-11 structure vs. unit-volume (2 f.u.) for (a) static energy, (b) $T$ = 0 K Helmholtz free energy including zero-point motion, and (c) $T$ = 300 K Helmholtz free energy. The difference between (a) and (b) corresponds to the zero-point energy contribution, and the difference between (b) and (c) corresponds to the 300 K thermal contribution.

TABLE S1. Proton sites in different supercell configurations.

| | Space group | Proton sites (2 GPa) |
|---|---|---|
| HOC-11 | $P2_1nm$ (primitive cell) | 2a (x, y, 0), (x + 1/2, -y, 1/2); |
| HOC-11* | $P2_12_12_1$ | 4a (x, y, z), (-x+1/2, -y, z + 1/2), (-x, y + 1/2, -z + 1/2), (x + 1/2, -y + 1/2, -z) |
| HOC-12 | Pm | 2c (x, y, z), (x, y, -z) |
| HOC-22 | $Pn2_1m$ (primitive cell) | 2a (x, y, 0), (-x, y+1/2, 1/2); |

# REFERENCE


[1] A. Sano-Furukawa, H. Kagi, T. Nagai, S. Nakano, S. Fukura, D. Ushijima, R. Iizuka, E. Ohtani, and T. Yagi, *Change in Compressibility of δ-AlOOH and δ-AlOOD at High Pressure: A Study of Isotope Effect and Hydrogen-Bond Symmetrization*, Am. Mineral. **94**, 1255 (2009).

[2] T. Kuribayashi, A. Sano-Furukawa, and T. Nagase, *Observation of Pressure-Induced Phase Transition of δ-AlOOH by Using Single-Crystal Synchrotron X-Ray Diffraction Method*, Phys. Chem. Miner. **41**, 303 (2014).

[3] A. Suzuki, *High-Pressure X-Ray Diffraction Study of ε-FeOOH*, Phys. Chem. Miner. **37**, 153 (2010).

[4] D. Simonova, E. Bykova, M. Bykov, T. Kawazoe, A. Simonov, N. Dubrovinskaia, and L. Dubrovinsky, *Structural Study of δ-AlOOH Up to 29 GPa*, Minerals **10**, 12 (2020).

[5] A. Sano-Furukawa, T. Hattori, K. Komatsu, H. Kagi, T. Nagai, J. J. Molaison, A. M. dos Santos, and C. A. Tulk, *Direct Observation of Symmetrization of Hydrogen Bond in δ-AlOOH under Mantle Conditions Using Neutron Diffraction*, Sci. Rep. **8**, 15520 (2018).

[6] H. Kagi, D. Ushijima, A. Sano-Furukawa, K. Komatsu, R. Iizuka, T. Nagai, and S. Nakano, *Infrared Absorption Spectra of δ-AlOOH and Its Deuteride at High Pressure and Implication to Pressure Response of the Hydrogen Bonds*, J. Phys. Conf. Ser. **215**, 012052 (2010).
